# Supplementary material for: QASnowball: An Iterative Bootstrapping Framework for High-Quality Question-Answering Data Generation
Source: arXiv:2309.10326 source file (2023-09-20)
Supplement: Supplementary file 1 [file 10_appendix.tex]

\appendix
\section{Appendix}
\label{sec:appendix}

implementation details
\subsection{Implementation Details}
\paragraph{Answer Extractor}
For Chinese pipeline, we use bert-wwm-base for training our answer extractor, with a batch size of 64, a constant learning rate of 1e-5, a weight decay of 1e-4 for 3 epochs. For English pipeline, we use bert-base instead, and the training settings is the same as described above.
\paragraph{Question Generator}
For Chinese pipeline, we use Mengzi-base for training our question generator, with a batch size of 10, a constant learning rate of 1e-5, a weight decay of 1e-4 for 5 epochs. For English pipeline, we directly use valhalla/t5-base-qa-qg-hl from huggingface/modelhub, which is fine-tuned on squad1.0 as our question generator.
\paragraph{QA-pair Filter}
For Chinese pipeline, we use pert-base for training our QA-pair filter. For English pipeline, we use pert-base-en. During training a fliter, all fine-tuning stages use a batch size of 32,  a maximum learning rate of 5e-5 with warm-up for the first 10 \% of training
and a weight decay of 0.0001. All pre-training stages use a batch size of 512, a maximum learning rate of 1e-5 with warm-up for the first 10 \% of training and a weight decay of 0.0001.
\noindent

\begin{table*}[!htb]
  \centering
    \begin{tabular}{l l cc cc cc cc}
    \hline
    \textbf{Model} & \textbf{Fine-tune} & \multicolumn{2}{c}{\textbf{CMRC}} &
             \multicolumn{2}{c}{\textbf{SQuAD-zh}} & \multicolumn{2}{c}{\textbf{DRCD}} & 
             \multicolumn{2}{c}{\textbf{DuReader}}\\
              & &EM & F1 & EM & F1 & EM & F1 & EM & F1\\ 
    \hline
    $PERT_{raw_{5M}}$ & in-domain     & 72.3  & 89.8  & 60.7  & 77.3  & 89.5    & \textbf{94.4}  & \textbf{75.9}  & 86.8 \\
    $PERT_{iter0_{5M}}$ & in-domain     & \textbf{73.4}  & \textbf{90.1}  & \textbf{60.8} & \textbf{77.4} & \textbf{89.5} & 94.3 & \textbf{75.7} & \textbf{86.8} \\
    \hline
    $PERT_{raw_{5M}}$ & seeds     & \textbf{72.5} & \textbf{89.4} & \textbf{60.4}  & \textbf{76.7}  & \textbf{76.1}    & \textbf{87.9}  & 74.3  & 86.0 \\
    $PERT_{iter0_{5M}}$ & seeds     & 71.1 & 88.8 & 60.2  & 76.6  & 73.4    & 86.0  & \textbf{75.4}  & \textbf{86.5} \\
    \hline
    \end{tabular}%
    \caption{\label{filter-raw-comparison}
Fine-tune experiments results(\%) for raw and filted data comparison. Seed fine-tune means model is fine-tuned on respective training set and tested on respective development set, which can be regarded as single task learning. Mix fine-tune means model is fine-tuned on a mix of datasets includes CMRC, SQuAD-zh and DuReader training set, which might be considered as multi-task learning.
}
\end{table*}


\begin{table*}[!htb]
  \centering
    \begin{tabular}{p{10cm}|p{2cm}|p{2cm}}
    \hline
    \textbf{Passage} & \textbf{Question} & \textbf{Analysis}\\
    \hline
   \begin{CJK}{UTF8}{gbsn}探讨电视胸腔镜辅助小切口手术(vamt)在自发性气胸治疗中的应用价值。\colorbox{green}{方法是}\colorbox{yellow}{于患侧腋中线第6或第7肋间置入胸腔镜套管} \colorbox{green}{，在靠近病变位置做长约5~8cm切口经肋间进胸(多在腋} \colorbox{green}{前线或腋中线第4~5肋)，使用普通手术器械与胸腔镜手术} \colorbox{green}{器械，在胸腔镜和直视下进行操作。}\end{CJK}
        
        \textbf{Translation}: Discussion of small incision hand assisted by video-assisted thoracoscopic
Application value of surgery (vamt) in the treatment of spontaneous pneumothorax
value. \colorbox{green}{Methods A} \colorbox{yellow}{thoracoscopic cannula was placed in the 6th or 7th intercostal} \colorbox{yellow}{space on the midaxillary line of the affected side} \colorbox{green}{, make an incision about 5-8cm long near the lesion and enter the} \colorbox{green}{chest through the intercostal area (mostly in the axilla) 4th to 5th} \colorbox{green}{ribs on the front line or midaxillary line), using common surgical} \colorbox{green}{ instruments and thoracoscopic surgery Instruments, operated} \colorbox{green}{ under thoracoscopic and direct vision.}& \begin{CJK}{UTF8}{gbsn}电视胸腔镜辅助小切口手术的方法是什么?
     
     What is the method of video-assisted thoracoscopic small incision surgery?\end{CJK} & \begin{CJK}{UTF8}{gbsn}Iteration 1 is able to extract longer answers\end{CJK}    \\
    \hline
    \begin{CJK}{UTF8}{gbsn}\colorbox{green}{民族主义可怕性的一面以及欧洲人对和平和繁荣的追求成为} \colorbox{green}{战后一体化的基本动因。民族主义对于欧洲一体化的作用在} \colorbox{green}{于它既是制约力量又是推动力量。一体化}\colorbox{yellow}{是民族主义与联} \colorbox{yellow}{邦主义相互作用}的结果。在民族国家占据一体化主导地位的情况下，一体化的发展还有相当的局限性。\end{CJK} 
    
    \textbf{Translation}: \colorbox{green}{The dire aspect of nationalism and the European} \colorbox{green}{quest for peace and prosperity became the basic motivation of} \colorbox{green}{postwar integration. The role of nationalism in European integra-} \colorbox{green}{tion is becauseit is both a restrictive force and a driving force} \colorbox{green}{integration} \colorbox{yellow}{is nationalism and union
The result of the interacti-} \colorbox{yellow}{on of nationalism.} Integrative dominance of the nation-state
Under the circumstances, the development of integration still has considerable limitations.
    & \begin{CJK}{UTF8}{gbsn}是什么导致了欧洲的一体化？\end{CJK} 

    What led to the integration of Europe?
    & \begin{CJK}{UTF8}{gbsn}Iteration 1 is able to extract longer answers\end{CJK}    \\
    \hline
    \begin{CJK}{UTF8}{gbsn}结果获取的雪旺细胞\colorbox{red}{纯度大于}\colorbox{yellow}{96\%};s-100免疫荧光鉴定细胞为阳性。结论本方法可以简单而快速地获得高纯度雪旺细胞。\end{CJK} 

    \textbf{Translation}: As a result, the purity of the obtained Schwann cells was \colorbox{red}{greater than} \colorbox{yellow}{96\%}; s-100 immunofluorescence identification cells are positive. Conclusion This method can obtain high-purity Schwann cell.
    & \begin{CJK}{UTF8}{gbsn}雪旺细胞的纯度是多少？\end{CJK} 

    What's the purity of Schwann cells?
    & \begin{CJK}{UTF8}{gbsn}Iteration 1 sometimes miss the important information about range\end{CJK}    \\
    \hline
    \end{tabular}%
    \caption{\label{filter-score-comparison}
Examples of iter0 and iter1 answers. Green color box texts indicates iteration 1 extracted answer, red color box texts indicate the iteration 0 answer, yellow color box texts indicates the overlapping texts. Translation is done by google Translate.
}
\end{table*}


\begin{table*}[!htb]
  \centering
    \begin{tabular}{p{8cm}|p{6cm}}
    \hline
    \textbf{Passage} & \textbf{Explanation}\\
    \hline
    \begin{CJK}{UTF8}{gbsn}因此，保护和发展森林资源便\colorbox{green}{成}\colorbox{yellow}{为改善生态}\colorbox{green}{环境}的重点工作。\end{CJK} 
    
    \textbf{Translation}: Therefore, the protection and development of forest resources has \colorbox{green}{be}\colorbox{yellow}{-come the focus of improving the ecological} \colorbox{green}{environment}.
    & our NER model inspect that  \begin{CJK}{UTF8}{gbsn}'为'(come) \end{CJK} should be contained in the entity \begin{CJK}{UTF8}{gbsn}'成为'(come) \end{CJK}, and similarly, \begin{CJK}{UTF8}{gbsn}'生态环境'(ecological environment) should appear as one entity, specially '生态'(ecology) could be viewed as noun. when it appears alone in chinese, and we detect '环境'(environment) is also a noun., thus they should be combined together.\end{CJK}\\
    \hline
    \begin{CJK}{UTF8}{gbsn}《河南社会科学》是河南省社会科学界联合会主办的\colorbox{green}{社会}\colorbox{yellow}{科学综合性学术}\colorbox{green}{刊物}，创刊于1993年10月，面向全国公开发行。\end{CJK} 
    \textbf{Translation}: "Henan Social Science" is a \colorbox{green}{social} \colorbox{yellow}{science comprehensive academic}\colorbox{green}{journal} sponsored by the Henan Provincial Federation of Social Science Circles. It was founded in October 1993 and is open to the public throughout the country.
     & our NER model inspect that  \begin{CJK}{UTF8}{gbsn}'科学'(science) \end{CJK} should be contained in the entity \begin{CJK}{UTF8}{gbsn}'社会科学'(social science) \end{CJK}, and similarly, \begin{CJK}{UTF8}{gbsn}'学术刊物'(academic journal) should appear as one entity, specially '学术'(academy) could be viewed as noun. when it appears alone in chinese, and we detect '刊物'(journal) is also a noun., thus they should be combined together.\end{CJK} \\

    \hline

    \begin{CJK}{UTF8}{gbsn}讨论了绿色供应链决策设施模型的\colorbox{yellow}{目标和约束条件，并提出} \colorbox{green}{模糊集}来描述不确定性。\end{CJK} 
    
    \textbf{Translation}: Discuss the green supply chain decision-making facility model's \colorbox{yellow}{objectives and constraints, and propose} \colorbox{green}{a fuzzy set} to describe the uncertainty.
    &  \begin{CJK}{UTF8}{gbsn}'提出'(propose) is a transitive verb and thus should not appear to be the end of the answer span, and thus we expand it into '提出模糊集'(propose a fuzzy set).\end{CJK}\\ \\
    \hline
    \end{tabular}%
    \caption{\label{filter-score-comparison}
Examples of post-processing in the answer extraction process. Green color box texts indicate parts of the final extract answer span, and yellow color box texts indicate the overlapping texts as well as the origin extracted answer span. Translation is done by google Translate.
}
\end{table*}


% filter case
\begin{table*}[!htb]
  \centering
    \begin{tabular}{p{7cm}|p{2cm}|p{2cm}|p{2cm}}
    \hline
    \textbf{Passage} & \textbf{Question} & \textbf{Category} & \textbf{Analysis}\\
    \hline
   \begin{CJK}{UTF8}{gbsn}背景原理天然铀矿包含三种同位素：大部分(99.274\%)为铀238，\colorbox{red}{约}\colorbox{yellow}{0.72}\colorbox{green}{\%}的铀235以及约0.0055\%的铀234。如果天然铀被提纯到包含3\%的铀235，那么就可以被轻水反应堆用作燃料。如果u-235的成分被提纯到90\%，则可被用来制作核武器。\end{CJK}
        
        \textbf{Translation}: Background Principles Natural uranium ore contains three isotopes: mostly (99.274\%) uranium 238, \colorbox{red}{about}\colorbox{yellow}{0.72}\colorbox{green}{\%} uranium 235 and About 0.0055\% uranium 234. If natural uranium is purified to contain 3\% uranium-235, it can be used as fuel in light water reactors. If the composition of u-235 is purified to 90\%, it can be used to make nuclear weapons
        & \begin{CJK}{UTF8}{gbsn}铀235含有多少百分比的铀235？ \end{CJK} What percentage of uranium 235 does uranium 235 contain?
        & \begin{CJK}{UTF8}{gbsn} filter's answer on the right\end{CJK}
        & \begin{CJK}{UTF8}{gbsn} Combining two answers gets better answer.\end{CJK}    \\
    \hline
    \begin{CJK}{UTF8}{gbsn}历史朱诺山因开矿而变得陡峭，1881年的时候它就被矿工叫做\colorbox{green}{金山}(\colorbox{red}{goldmountain})，1896年又出现秃山(baldmountain)的称呼，朱诺山一名出现在1888年。\end{CJK} 
    
    \textbf{Translation}: History Juno Mountain became steep due to mining. In 1881, it was called \colorbox{green}{Gold Mountain} (\colorbox{red}{goldmountain}) by miners. In 1896, it was called Bald Mountain (baldmountain) again. , the name Juno Mountain appeared in 1888.
    & \begin{CJK}{UTF8}{gbsn}朱诺山的矿工叫什么名字？\end{CJK} What was the miner's name on Mount Juno?
    & \begin{CJK}{UTF8}{gbsn} no overlap\end{CJK}
    & \begin{CJK}{UTF8}{gbsn} A good example for filtering no overlapping answers.\end{CJK}    \\
    \hline
    \begin{CJK}{UTF8}{gbsn}化古埃及人将粪金龟(推粪虫、屎壳郎)视为生命永恒的象征，因为其推动粪球有如太阳东升西落运转一般，象征埃及太阳神拉。经济重要性许多种类会对经济植物造成危害。如在北美危害\colorbox{green}{花卉、果树、}\colorbox{yellow}{农作物}\colorbox{red}{的日本豆金龟}。粪金龟能分解动物的粪便，因此在非洲和澳洲的生态上扮演重要的角色。\end{CJK} 

    \textbf{Translation}: The ancient Egyptians regarded the dung beetle (dung beetle, dung beetle) as a symbol of eternal life, because it pushed the dung ball like the sun rising in the east and setting in the west, symbolizing the Egyptian sun god Ra. Economic importance Many species can cause damage to economic plants. For example, in North America, \colorbox{green}{flowers, fruit trees,}\colorbox{yellow}{crops}\colorbox{red}{bean beetles} are endangered. Dung beetles play an important role in the ecology of Africa and Australia as they decompose animal feces.
    & \begin{CJK}{UTF8}{gbsn}粪金龟在北美危害什么？\end{CJK}  What do dung beetles do in North America?
    & \begin{CJK}{UTF8}{gbsn} filter's answer on the left\end{CJK}
    & \begin{CJK}{UTF8}{gbsn}Sometimes merge some irrelated information into the answer.\end{CJK}    \\
    \hline
    \end{tabular}%
    \caption{\label{filter-score-comparison}
Examples of origin answers before a filter, filter's answer and new answers after a filter. Green color box texts indicates filter's answer, red color box texts indicate the origin answer, yellow color box texts indicates the overlapping texts. Translation is done by google Translate.
}
\end{table*}


\begin{table*}[!htb]
  \centering
    \begin{tabular}{|l|l|l|l|}
    \hline
    \textbf{total test} & \textbf{wrong data} & \textbf{iter0 better} & \textbf{iter1 better}\\
    \hline
    200 & 46 & 38 (24.7\%) & 116(75.3\%)\\
    \hline
    \end{tabular}%
    \caption{\label{filter-score-comparison}
Human annotated comparison between the different parts from iteration 0 and iteration 1 QA-pairs.
}
\end{table*}

\begin{table*}[!htb]
  \centering
    \begin{tabular}{l l l l l l}
    \hline
    \textbf{Data Source} & \textbf{Iteration} & \textbf{Data Amount} & \textbf{Pass Rate} & \textbf{Strong Example Recall}\\
    \hline
    Part 3 & 0 & 500k & 73\% & 53.1\%\\
    & 1 & 472k & 82\% & 66.7\%\\
    & 2 & 475k & 86\% & 73.7\%\\
    \hline
    \end{tabular}%
    \caption{\label{filter-score-comparison}
Human evaluation on the proportion of data of satisfying quality from different iterations. We believe that our method is better than the score-based filtering methods, so we calculate the percentage of qualified data among those with scores below a certain threshold. We focus on how much correct data can we extract from the filter's predictions, especially from that their scores are below a certain threshold. We set the threshold to the average score overall average score in one split of evaluation data, Part 3 Iteration 0 e.g., because we find that the data above this threshold and the data below this threshold are roughly divided into 70\% and 30\%. This allows for maximum simulation of data quality when using score-based filtering methods.
}
\end{table*}


\begin{figure*}[htbp]
  \begin{minipage}{0.45\textwidth}
    \includegraphics[width=\textwidth]{figs/DRCD EM.png}
    \caption{Few shot results for DRCD exact match/}
  \end{minipage}
  \hspace{0.05\textwidth}
  \begin{minipage}{0.45\textwidth}
    \includegraphics[width=\textwidth]{figs/DRCD F1.png}
    \caption{Few shot results for DRCD F1 rate}
  \end{minipage}

  \begin{minipage}{0.45\textwidth}
    \includegraphics[width=\textwidth]{figs/TriviaQA EM.png}
    \caption{Few shot results for TriviaQA exact match}
  \end{minipage}
  \hspace{0.05\textwidth}
  \begin{minipage}{0.45\textwidth}
    \includegraphics[width=\textwidth]{figs/TriviaQA F1.png}
    \caption{Few shot results for TriviaQA F1 rate}
  \end{minipage}
  \caption{Illutration of the few-shot experiment results}
  \label{fig:my_label}
\end{figure*}

\begin{figure*}[htbp]
  \begin{minipage}{0.45\textwidth}
    \includegraphics[width=\textwidth]{figs/bar-plot-EM.png}
    \caption{Zero-shot experiments results on different datasets/}
  \end{minipage}
  \hspace{0.05\textwidth}
  \begin{minipage}{0.45\textwidth}
    \includegraphics[width=\textwidth]{figs/bar-plot-f1.png}
    \caption{Zero-shot experiments results on different datasets}
  \end{minipage}

  \begin{minipage}{0.45\textwidth}
    \includegraphics[width=\textwidth]{figs/bar-plot-EM-en.png}
    \caption{Zero-shot experiments results on different datasets/}
  \end{minipage}
  \hspace{0.05\textwidth}
  \begin{minipage}{0.45\textwidth}
    \includegraphics[width=\textwidth]{figs/bar-plot-F1-en.png}
    \caption{Zero-shot experiments results on different datasets}
  \end{minipage}

\end{figure*}
